# Supplementary material for: Neurodegenerative damage reduces firing coherence in a continuous attractor model of grid cells
Source: arXiv:2008.05591 ancillary file (2021-04-14)
Supplement: Supplementary file 1 [file supporting_information-3.pdf]

# Supporting Information

## Contents


**1 Influence of Time Steps $dt$ for Accelerating Simulation** **2**

**2 Explanation of Flow Determined by Preferred Direction and Shifted Location Vectors** **2**

**3 Influence of Velocity Input Coefficient** **3**

**4 Mean Field Analysis to Explain Triangular Grids** **4**

**5 Aperiodic Boundary Conditions** **6**

**6 Influence of Increasing Length for Path Integration Map** **7**

# 1 Influence of Time Steps $dt$ for Accelerating Simulation

To improve simulation effectiveness, we found the time step $dt$ plays a big part in simulation speed. A bigger time steps $dt$ means less numerical simulating cycles within the same period of time. A small time step $dt$ can improve the simulation accuracy; we find that larger time steps can also generate the hexagonal grid structure. In particular, $dt = 0.5, 1.0, 2.0ms$ can each generate a hexagonal lattice grid for a long enough animal trajectory as shown in Fig. 1. Accordingly, we sacrifice some accuracy for better simulation speed by choosing a larger $dt$, which can still get us good results for average path integration maps.

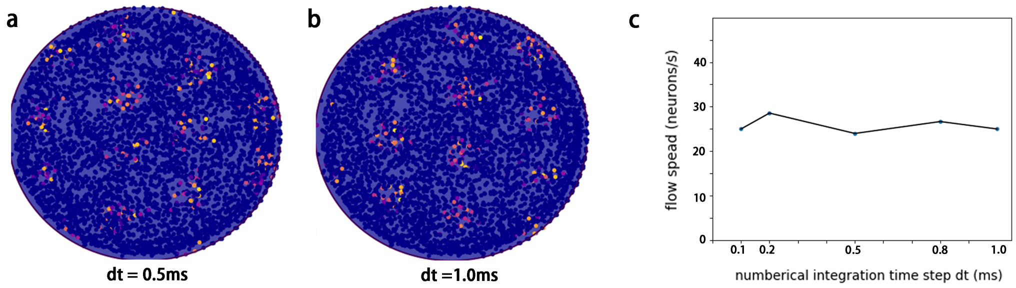


Figure 1: **Influence of time step size $dt$ on simulations.** (a) Average path integration map of Neuron # 800, healthy grids, dt = 0.5ms. (b) Neuron # 800, healthy grid, dt = 1.0ms. (c)different time steps $dt = 0.1ms, 0.2ms, 0.5ms, 0.8ms, 1.0ms$ don't affect the flowing speed when velocity inputs are the same ($\vec{v} = 1m/s$)

# 2 Explanation of Flow Determined by Preferred Direction and Shifted Location Vectors

The grid cells can create a grid like firing pattern without the shifted location vectors $l\hat{e}_{\theta_j}$, but the inclusion of $l\hat{e}_{\theta_j}$ is the key to generate a steady firing pattern flow. The addition of $l\hat{e}_{\theta_j}$ breaks the symmetry of weight matrix $W$ to make $W_{ij} \neq W_{ji}$ between two neurons. In Fig. 2a,b, all the neurons have the same preferred direction $\hat{e}_{\theta_j}$ to the right, and the new weight matrix $W_{ij}(x_i - x_j - l\hat{e}_{\theta_j})$ is bigger in magnitude than $W_{ji}(x_j - x_i - l\hat{e}_{\theta_i})$ considering $l\hat{e}_{\theta_i} = l\hat{e}_{\theta_j}$. Because weight matrix is negative, the connection along the preferred direction has bigger inhibitory affects than the connection in the opposite direction, which drives the grid-like firing pattern move opposite the preferred direction. When neuron groups with different preferred directions $\hat{e}_{\theta_j}$ work together equally, the symmetry of the weight matrix can be restored and that explains why there is a static firing pattern when the velocity input is zero(Fig. 2c). When the velocity input is nonzero, it can strongly activate the neurons that share the same preferred direction, which drives the grid-like firing pattern to flow in the opposite direction to the velocity.

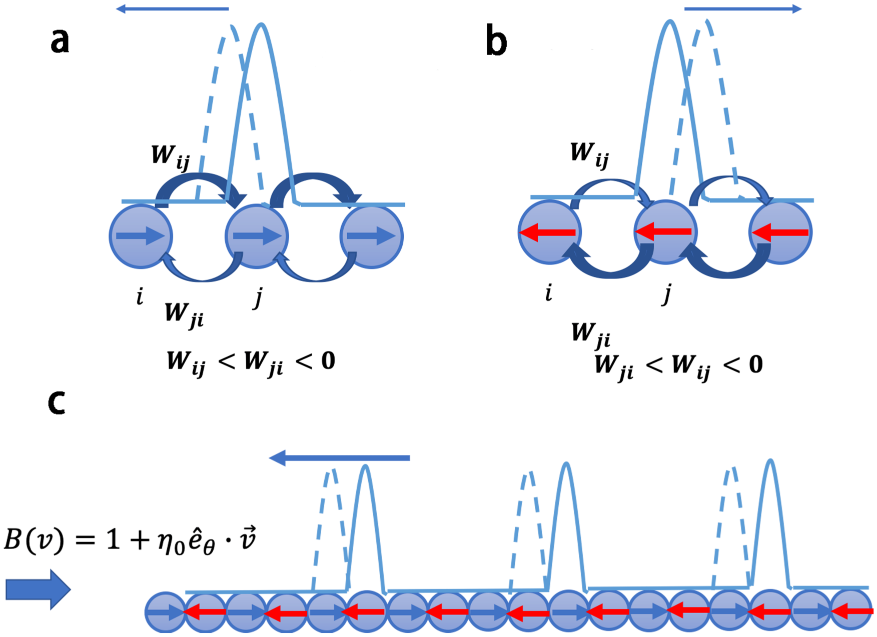


Figure 2: **1D Grid cell Model with Preferred Direction.** (a) Neurons have preferred direction pointing to the right, breaking the symmetry of weight matrix($W_{ij} < W_{ji} < 0$), the inhibitory connection to left is bigger than that to the right, which drives the grids firing pattern to move to the left. The blue arrow indicates driving flow direction, the solid blue curve is current firing pattern and the dashed curve indicates the firing signal the next moment. (b) Neurons with preferred direction pointing to the left drive the flow pointing to the right. (c) neurons with different preferred directions work together evenly make the grid-like pattern stationary, and with non-zero velocity input pointing to the left(big blue arrow) will drive the grids to flow to the left.

## 3 Influence of Velocity Input Coefficient

$\eta_0$ is the coefficient that characterizes the effects of velocity inputs to the driven pattern flow, and in the paper we have it to be 0.10315. It controls the gain from velocity to the feed-forward input **B**. $\eta_0$ can be used to determine the driving force from rat's velocity, and under the same rat's velocity, a bigger $\eta_0$ can drive the flow faster, and in Fig. 3, it shows a linear relationship between $\eta_0$ and flow speed. Also, the larger variance with increasing $\eta_0$ proves that we want to choose $(|\eta_0 \hat{e}_{\theta_j} \cdot \vec{v}| \ll 1)$ to keep the formed lattice stable.

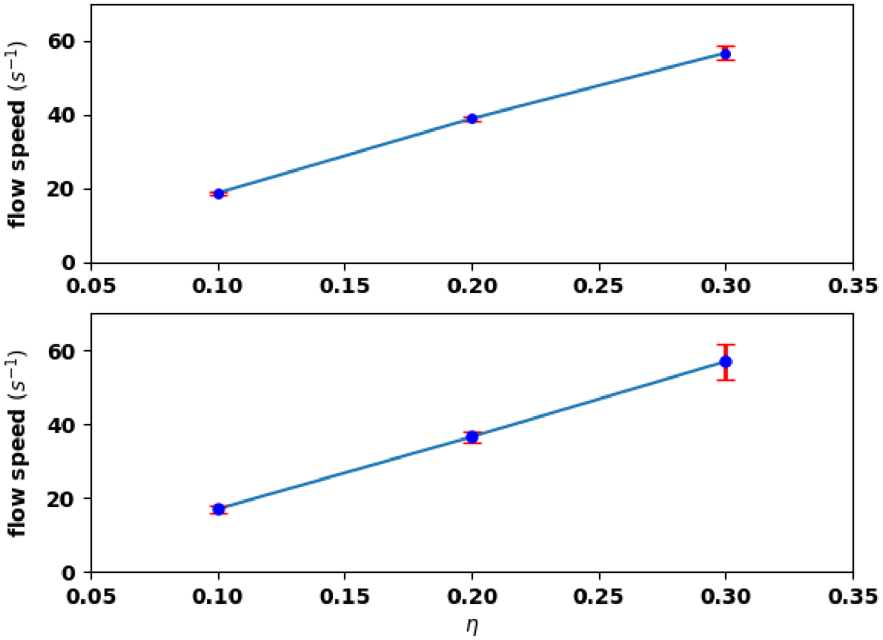


Figure 3: **Linear relationship between flow speed and velocity input coefficient** $\eta_0$ Top: healthy neuron sheet, with input velocity to be 0.7 $m/s$. Bottom: damaged neuron sheet ($R = 7, \alpha = 0$), the same input velocity. The red error bars are the variance.

# 4 Mean Field Analysis to Explain Triangular Grids

The firing rate equations for Burak and Fiete are:

$$\tau \frac{ds_i}{dt} = -s_i + f\left(\sum W_{ij} \cdot s_i + B_i\right) \tag{1}$$

where:

$$W_{ij} = e^{-\gamma|\vec{x}_i - \vec{x}_j|} - e^{-\beta|\vec{x}_i - \vec{x}_j|} \tag{2}$$

with $w_{ij} < 0$ uniformly and $s_i > 0, B = 1$. There is no region of $s_i$ space where the argument of the rectification in $(C1)$ is negative hence $(C1)$ is always in the linear regime.

The fixed point is set by the condition

$$\frac{ds_i}{dt} = 0 \tag{3}$$

with $s_i = \sum W_{ij} \cdot s_i + B$ which can be viewed as the solution arising from minimizing the "cost function"

$$C(s_i) = \frac{1}{2}\sum {s_i}^2 - \sum B \cdot s_i - \frac{1}{2} s_i W_{ij} s_j \quad . \tag{4}$$

Fourier transformation of the firing rates is given by

$$s_i = \frac{1}{\sqrt{N}} \sum \tilde{s}(\tilde{q}) e^{-i \cdot \tilde{q} \cdot r_i} \tag{5}$$

$\vec{r}_i$ is the neuron position in $N \times N$ sheets; $\vec{r}_i + N\hat{x} = \vec{r}_i + N\hat{y} = \vec{r}_i$. $\tilde{q} \subset [q_x, q_y]$,$-\frac{\pi(N-1)}{N} \leq q_\alpha \leq \pi$,$\alpha = x, y$. where

$$\widetilde{W}(\tilde{q}) = \frac{\pi}{\gamma} e^{-\frac{q^2}{4\gamma}} - \frac{\pi}{\beta} e^{-\frac{q^2}{4\beta}} \tag{6}$$

With $\widetilde{W}(\tilde{q}) > 1$, an instability at finite $\tilde{q}$ is possible. $\widetilde{W}(0) = \frac{\pi}{\gamma} - \frac{\pi}{\beta}$, and $\widetilde{W}(\tilde{q})$ is maximum when $\widetilde{q_0} = 2\sqrt{2(\frac{\beta\gamma}{\gamma-\beta}) \ln(\frac{\gamma}{\beta})}$.

We can assume different solutions of the form

$$s_i(\vec{r}) = a_i[1 + b_i \sum f_i(\widetilde{q_k} \cdot \vec{r})] \tag{7}$$

where $|\widetilde{q_k}| = q_0$, and there are constraints:
(1) $1 + b_i \sum f_i(\widetilde{q_k} \cdot \vec{r}) \geq 0$
(2) $f_i(\widetilde{q_k} \cdot \vec{r})$ must be periodic.
Examples are:
(1) $s_0(\vec{r}) = a_0$, uniformly.
(2) $s_1(\vec{r}) = a_1[1 + \cos(q_0 x)]$, periodical along x direction.
(3) $s_2(\vec{r}) = a_2[1 + \frac{1}{2}\cos(q_0 x) + \frac{1}{2}\cos(q_0 x)]$, orthorhombic grids.
(4) $s_3(\vec{r}) = a_3[1 + \frac{2}{3}\cos(\vec{q}_1\vec{r}) + \frac{2}{3}\cos(\vec{q}_2\vec{r}) + \frac{2}{3}\cos(\vec{q}_3\vec{r})]$, triangular grids.
where $\vec{q}_1 = q_0(1, 0)$, $\vec{q}_2 = q_0(-\frac{1}{2}, \frac{\sqrt{3}}{2})$, $\vec{q}_3 = q_0((-\frac{1}{2}, -\frac{\sqrt{3}}{2})$.

Their Fourier Transforms are
(1) $\widetilde{s_0}(\tilde{q}) = a_0 \delta_{\tilde{q},0}$
(2) $\widetilde{s_1}(\tilde{q}) = a_1[\delta_{\tilde{q},0} + \frac{1}{2}(\delta_{\tilde{q},q_0 x} + \delta_{\tilde{q},-q_0 x})]$
(3) $\widetilde{s_2}(\tilde{q}) = a_2[\delta_{\tilde{q},0} + \frac{1}{4}(\delta_{\tilde{q},q_0 x} + \delta_{\tilde{q},-q_0 x} + \delta_{\tilde{q},q_0 y} + \delta_{\tilde{q},-q_0 y})]$
(4) $\widetilde{s_3}(\tilde{q}) = a_3[\delta_{\tilde{q},0} + \frac{1}{3}(\delta_{\vec{q}_1 \cdot \vec{r}} + \delta_{-\vec{q}_1 \cdot \vec{r}} + \delta_{\vec{q}_2 \cdot \vec{r}} + \delta_{-\vec{q}_2 \cdot \vec{r}} + \delta_{\vec{q}_3 \cdot \vec{r}} + \delta_{-\vec{q}_3 \cdot \vec{r}})]$

Substituting these in the cost function yields the results

$$C[\widetilde{S}_{\tilde{q}}] = \frac{1}{2} \sum_{\tilde{q}} |\tilde{s}(\tilde{q})|^2 [1 - \widetilde{W}(\tilde{q})] - \sqrt{N} B \tilde{s}(\tilde{q} = 0) \tag{8}$$

(1) $C_0 = -\sqrt{N} B a_0 + \frac{{a_0}^2}{2}[1 - \widetilde{W}(0)]$
(2) $C_1 = -\sqrt{N} B a_1 + \frac{{a_1}^2}{2}\{[1 - \widetilde{W}(0)] + \frac{1}{2}[1 - \widetilde{W}(q_0)]\}$
(3) $C_2 = -\sqrt{N} B a_2 + \frac{{a_2}^2}{2}\{[1 - \widetilde{W}(0)] + \frac{1}{4}[1 - \widetilde{W}(q_0)]\}$
(4) $C_3 = -\sqrt{N} B a_3 + \frac{{a_3}^2}{2}\{[1 - \widetilde{W}(0)] + \frac{2}{3}[1 - \widetilde{W}(q_0)]\}$

We can summarize these results as:

$$C_i = -\sqrt{N}Ba_i + \frac{{a_i}^2}{2}\{[1 - \widetilde{W}(0)] + \sigma_i[1 - \widetilde{W}(q_0)]\} \tag{9}$$

Introducing

$$\rho_i = [1 - \widetilde{W}(0)] + \sigma_i[1 - \widetilde{W}(q_0)] \tag{10}$$

Equation (C9) can be changed into:

$$C_i = \frac{\rho_i}{2}\left(a_i - \frac{\sqrt{N}B}{\rho_i}\right)^2 - \frac{NB^2}{2\rho_i} \tag{11}$$

$$C_{i,\min} = -\frac{NB^2}{2\rho_i} \text{ when } a_i = \frac{\sqrt{N}B}{\rho_i}. \tag{12}$$

For a $40 \times 40$ neuron sheet with $a = 1$, $N = 1600$, $B = 1$, $\gamma = 6.7 \times \beta$, $\beta = \frac{3}{64}$; We have $\tilde{q}_0 = 0.916$, and $\widetilde{W}(0) = -57.02$, $\widetilde{W}(\tilde{q}_0) = 4.37$.
(1) $C_{0,\min} = -13.79, \quad a_0 = 0.689$
(2) $C_{1,\min} = -14.20, \quad a_1 = 0.71$
(3) $C_{2,\min} = -13.99, \quad a_2 = 0.6995$
(4) $C_{3,\min} = -14.34, \quad a_3 = 0.7172$

Notice that the hexagonal grid shows the lowest cost, indicating it is more stable than grid structures.

# 5 Aperiodic Boundary Conditions

the feed-forward input to neuron $i$ is:

$$B_i(x) = A_i(x)(1 + \eta_0 \hat{e}_{\theta_i} \vec{v}) \tag{13}$$

$A_i(x)$ is called the *envelope function* which helps to modulate the strength of the input to the neurons.

$$A(\vec{x}) = \begin{cases} 1 & |\vec{x}| < R - \mathit{\Delta} r \\ exp[-a_0(\frac{|\vec{x}| - R + \mathit{\Delta} r}{\mathit{\Delta} r})^2] & R - \mathit{\Delta} r \leq |\vec{x}| \leq R \end{cases} \tag{14}$$

$R = 20$ is the radius of the $40 \times 40$ network and $a_0 = 4$. $\mathit{\Delta} r$ determines the range of radius over which input tapering occurs, the larger $\mathit{\Delta} r$, the more gradual the tapering. In all aperiodic simulations, $\mathit{\Delta} r = R$. [Bruak. & Fiete.]

# 6 Influence of Increasing Length for Path Integration Map

To check the what happened when we use longer paths for simulation, we ran for 5× longer trajectories (500s) and present the result in Fig. 4. The healthy neuron sheets can generate a grid-like pattern and the damaged one loses its grid. Comparing with the method (in the main paper) of using the average of five independent shorter trajectories (100s), the results of those longer runs are similar to those of the shorter ones, so that an increasing length doesn't destroy or enhance the grid-like pattern in a healthy neuron sheet. We can say the path integration map is still stable within a long time range (up to 500s), and for the same damage situation ($\alpha = 0.8, R = 7$), we find similar loss of grid firing as for the shorter time runs. It is safe to conclude that the grid pattern loss is not eliminated by a longer path integration but the defects. Meanwhile, using an average of independent trajectories is more effective because we can do parallel simulations at the same time.

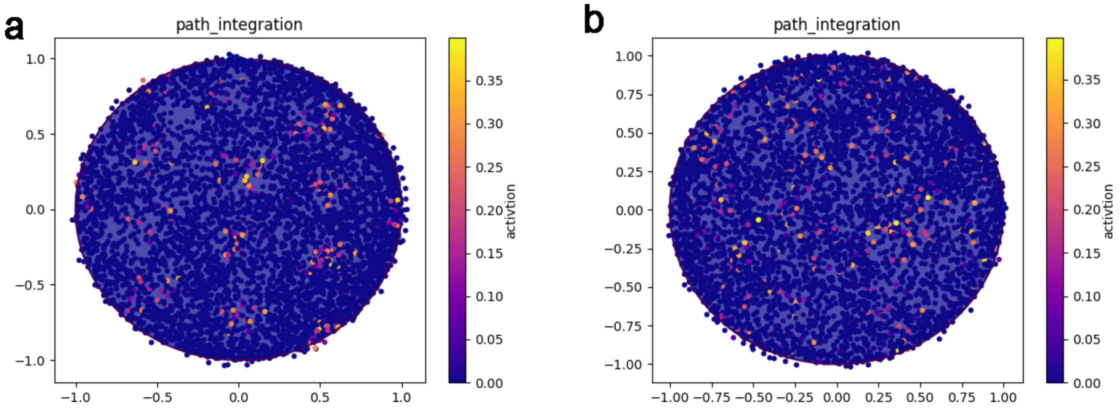


Figure 4: **Longer path integration maps of healthy and damaged neuron sheets** a, Healthy neuron sheets, 500s path integration map of neuron #800, b, Damaged neuron sheets ($\alpha = 0.8, R = 7$), 500s path integration map of neuron #800.
